# Supplementary material for: Rack Position Optimization in Large-Scale Heterogeneous Data Centers
Source: arXiv:2504.00277 source file (2025-03-31)
Supplement: Supplementary file 1 [file appendix.tex]

\section{A fast heuristic algorithm}

\begin{enumerate}
    \item Represent state with a base tensor X,  of dimension position by racktypes; where $X_{ij}=1$ if position $i$ is occupied by racktype $j$;
    \item Build a computational graph with $X$ at bottom, then resource utilization in all scopes, then penalizing resource utilization overage, and metrics representing the spread of certain resource utilization. Let the overall objective be a weighted sum of all overage nodes and spread quality nodes. Let the top node be $f$.
    \item When deciding where to place a rack of type $\bar{j}$, evaluate $\nabla f(X)$, then pick the position $i^*$ such that
    \[i^* = \arg\max\left\{i \ \middle| \ [\nabla f(X)]_{i,\bar{j}}\right\} \]
    \item Update $X_{i^* \bar{j}} \leftarrow X_{i^* \bar{j}} + 1$;
\end{enumerate}
